# Supplementary material for: CNN-based Dendrite Core Detection from Microscopic Images of Directionally Solidified Ni-base Alloys
Source: arXiv:2305.12506 source file (2023-05-21)
Supplement: Supplementary file 1 [file 7_Appendix.tex]

\chapter{The number of dendrite cores detected}

%-----------comparison----------------

\begin{table*}
\centering
\small
{\vspace{-500pt}
    \resizebox{1.0\linewidth}{!}{
    {
	\begin{tabular}{l|l|c|c|c}
		
    \toprule
     \multicolumn{1}{l|}{Methods} & \multicolumn{1}{l|}{deviation} & \multicolumn{1}{c|}{Total} & \multicolumn{1}{c|}{T-Positive$\uparrow$}  & \multicolumn{1}{c}{F-Positive$\downarrow$}  \\
   \midrule
   \multirow{1}{*}{SSD}                
      & 10  & 1882 & 1804 & 112\\
      %& 20  & 0.9659 & 0.9488 & 0.9573\\
      
    \midrule
    \multirow{1}{*}{Faster-RCNN}   
    & 10    & 1882 & 1715 & 180\\
    %& 20    & 0.9633 & 0.9567 & 0.9600\\

    \midrule
    \multirow{1}{*}{Stacked-Hourglass}   
     & 10   &  1882 & 1800 & 83\\
     
    \midrule
    \multirow{1}{*}{\topone{Ours}}   
     & 10  & 1882 & \topone{1814} & \topone{54}\\

    \bottomrule
		
	\end{tabular}
	}
	}
}
\vspace{-15pt}
\caption{Comparison results of \cite{liu2016ssd}, \cite{ren2015faster}, \cite{newell2016stacked}, and our method based on the number of dendrite cores detected.}
\label{tab:comparison_number}

\end{table*}
%---------------------------

%-----------------------------
\begin{table*}
\centering
\small
{
    \resizebox{1.0\linewidth}{!}{
    {
	\begin{tabular}{l|l|c|c|c}
		
    \toprule
     \multicolumn{1}{l|}{Methods} & \multicolumn{1}{l|}{deviation} & \multicolumn{1}{c|}{Total} & \multicolumn{1}{c|}{T-Positive$\uparrow$}  & \multicolumn{1}{c}{F-Positive$\downarrow$}  \\
   \midrule
   \multirow{1}{*}{ESDN}                
      & 10  & 1882 & 1800 & 83\\
      
    \midrule
    \multirow{1}{*}{+HSDN}   
    & 10    & 1882 & \topone{1820} & 83\\

    \midrule
    \multirow{1}{*}{\topone{+BCN}}   
     & 10  & 1882 &  1814 & \topone{54}\\

    \bottomrule
		
	\end{tabular}
	}
	}
}
\vspace{-15pt}
\caption{Ablation study on ESDN, HSDN, and BCN based on the number of dendrite cores detected. We show the result for ESDN at the first row, ESDN + HSDN at the second row and ESDN + HSDN + BCN at the third row. In the ablation study, we use the deviation 10 pixels.}
\label{tab:ablation_number}
\end{table*}
%------------------------------------------------
