# Supplementary material for: CNN-based Dendrite Core Detection from Microscopic Images of Directionally Solidified Ni-base Alloys
Source: arXiv:2305.12506 source file (2023-05-21)
Supplement: Supplementary file 2 [file 8_Appendix.tex]

\chapter{Exploit the crop size and crop intensity}
\label{crop_intensity}

%--------------------------------------------------------- Exploit the Crop size
\section{Exploit the crop size}
\label{subsec:crop}

\begin{figure}[h!]
  \includegraphics[width=1\textwidth]{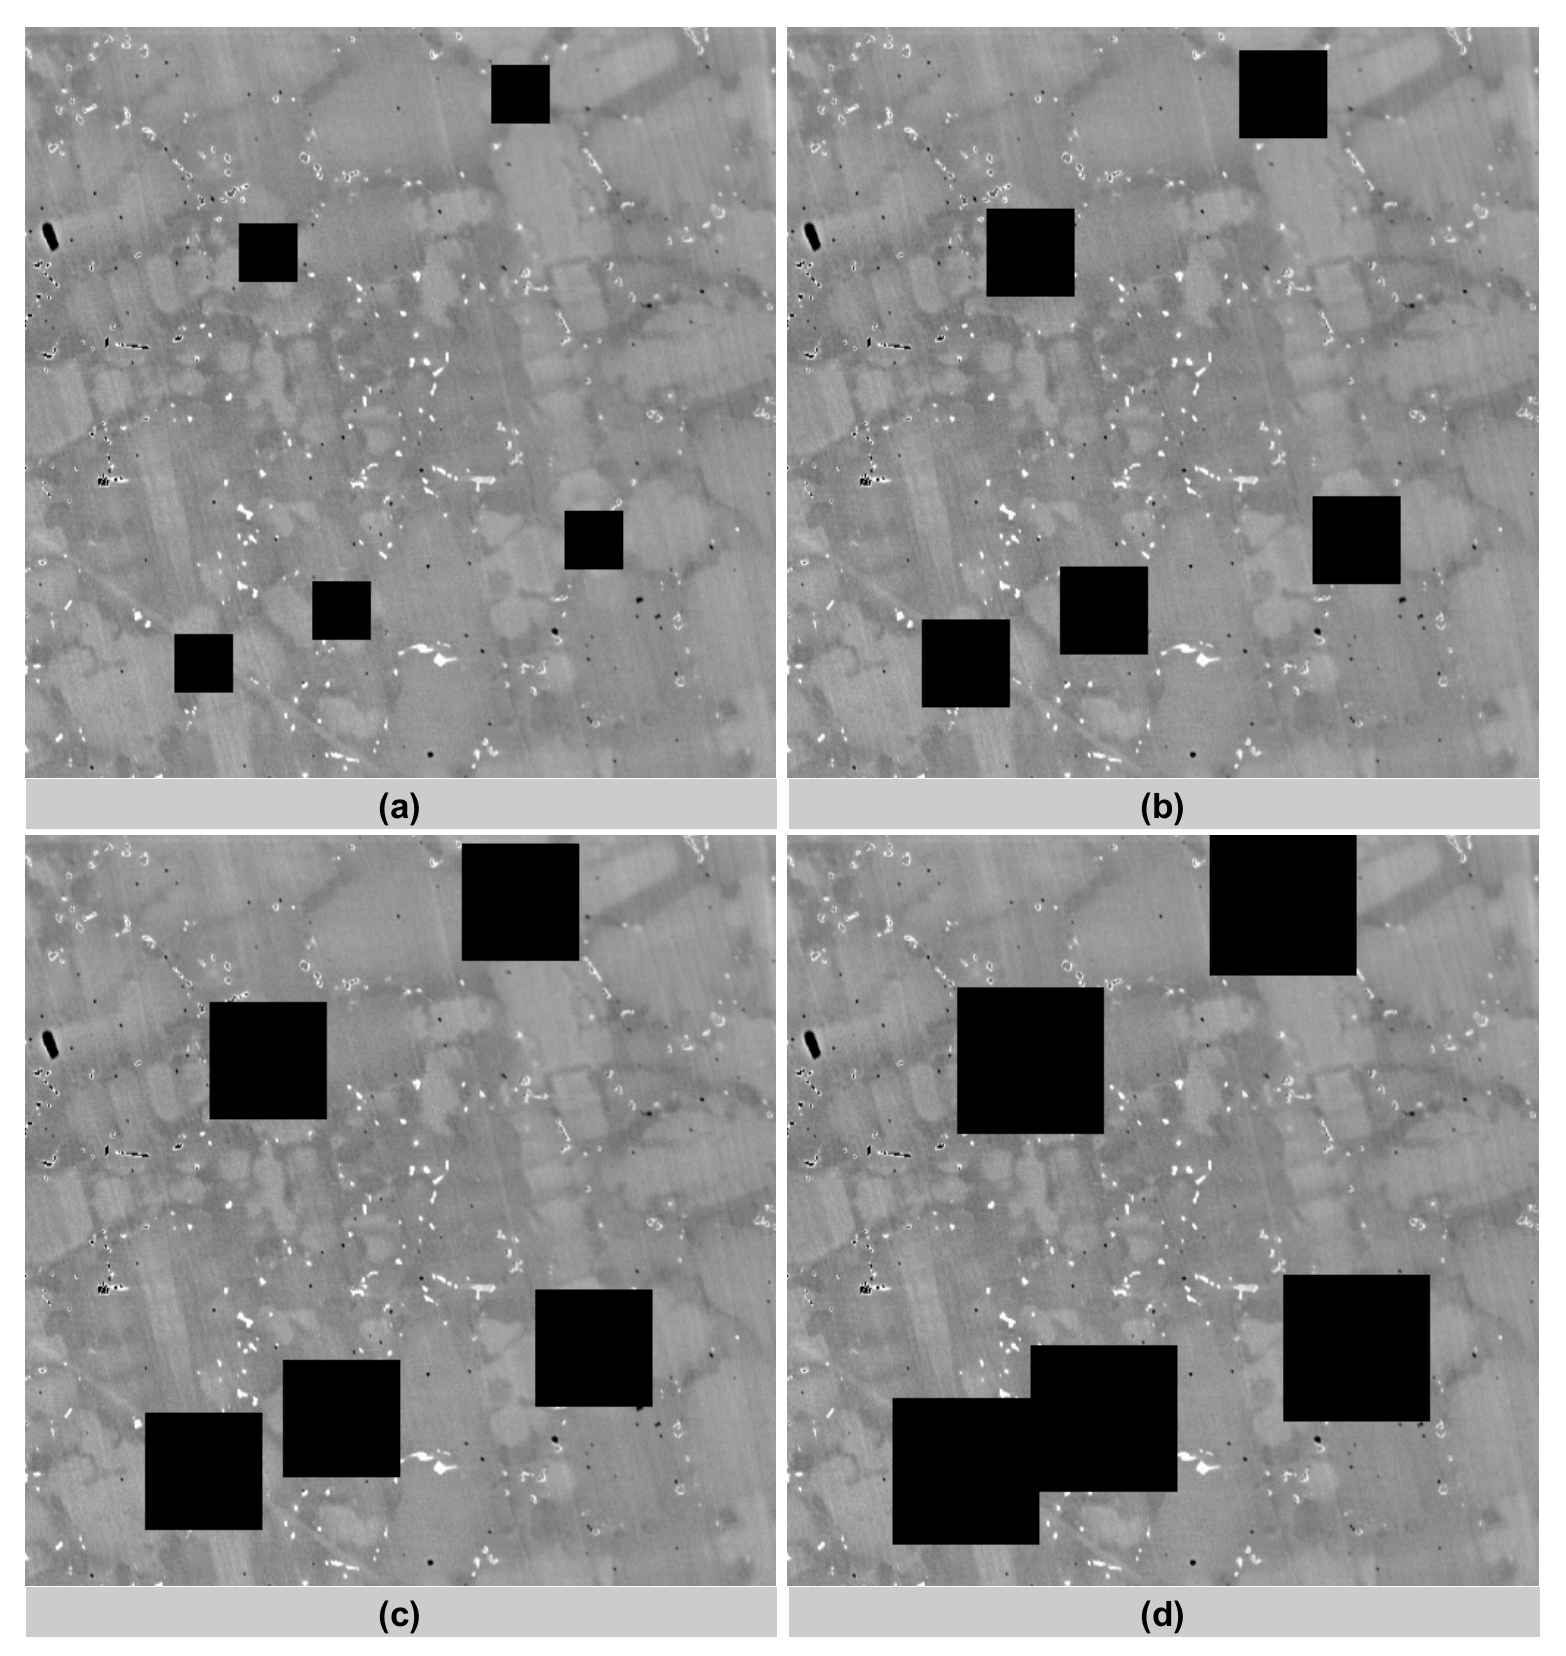}
  \vspace{-25pt}
  \caption{The visualization of different crop sizes. (a) denotes the crop size 40*40, (b) denotes the crop size 60*60, (c) denotes the crop size 80*80, and (d) denotes the crop size 100*100.}
  \label{fig:crop_size}
\end{figure}

During the procedure of destroying the structure of easy samples of dendrites detected by ESDN, the crop size is a big fact that can affect the final detected result. In order to exploit the reasonable crop size, we have conducted a series of experiments. We take different crop sizes to destroy the structure of easy samples of dendrites. Specifically, we use the crop size 40*40, 60*60, 80*80, 100*100, and no crop. The visualization results of the cropped images are displayed in \figref{fig:crop_size}. 

We evaluate the Recall, Precision, and F-score with different crop sizes and show the results in \tableref{tab:crop_size} and \figref{fig:crop_curve}. From \figref{fig:crop_curve}, we can see that \ding{182} Without destroying the structure of easy samples of dendrites detected by ESDN, the final F-score is very low. \ding{183} It reaches the best F-score when the crop size is 80*80. When continue to increase the crop size to 100*100, the F-score begins to decrease. The reason for this result is that the smaller crop size or without cropping can not destroy the structure of dendrites detected by ESDN and the larger crop size may destroy the potential dendrites which should be detected by HSDN. Based on these observations, we finally choose the crop size 80*80.

\begin{figure}[h!]
  \includegraphics[width=1\textwidth]{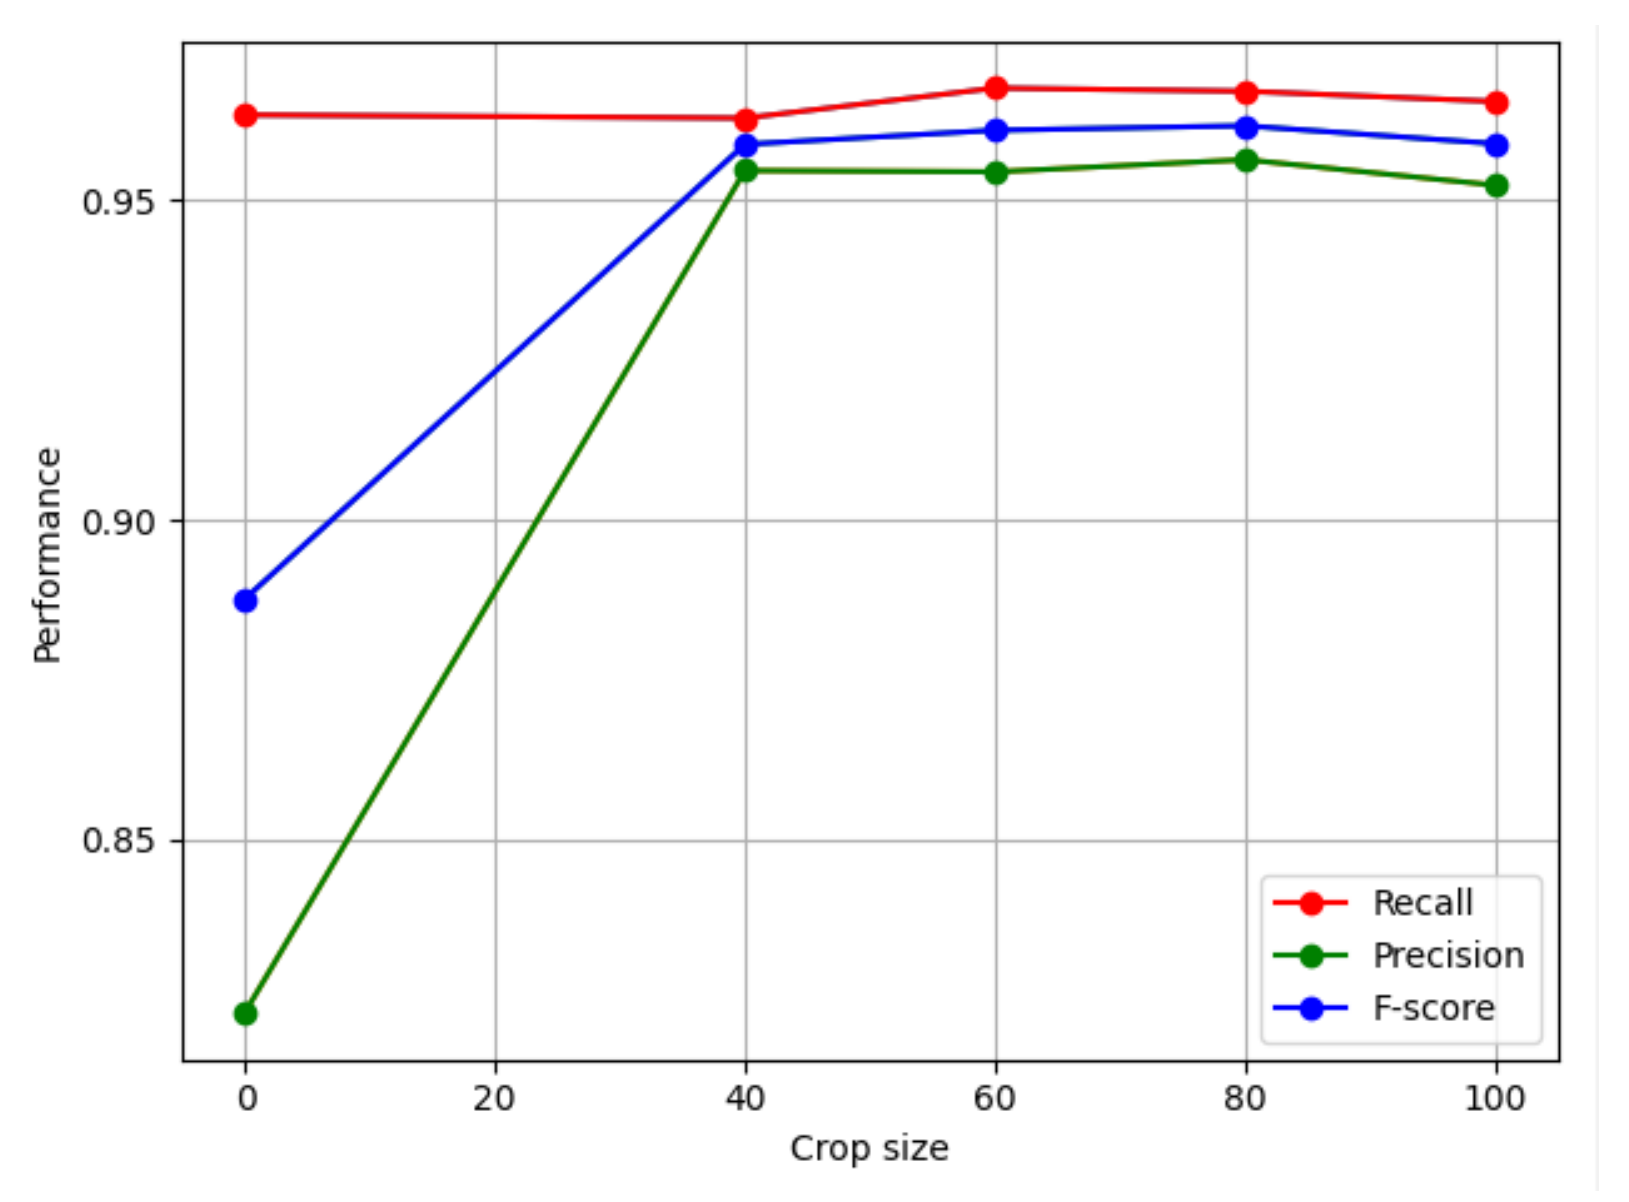}
  \vspace{-25pt}
  \caption{Exploiting the optimal crop size. Red points denote the Recall, green points denote the Precision, and blue points denote the F-score. When the crop size is equal to 80*80, it gets the best F-score.}
  \label{fig:crop_curve}
\end{figure}

%----------crop_size----------------
\begin{table*}
\centering
\small
{
    \resizebox{0.8\linewidth}{!}{
    {
	\begin{tabular}{l|c|c|c}
		
    \toprule
     \multicolumn{1}{l|}{Crop size} & \multicolumn{1}{c|}{Recall$\uparrow$} & \multicolumn{1}{c|}{Precision$\uparrow$}  & \multicolumn{1}{c}{F-Score$\uparrow$}  \\
     
   \midrule
                 
       no crop  & 0.9633 & 0.8229 & 0.8876\\
   
   \midrule
                
       40*40  & 0.9628 & 0.9546 & 0.9587\\
 
    \midrule
                
       60*60  & 0.9675 & 0.9544 & 0.9609\\

    \midrule
  
      \topone{80*80}  & \topone{0.9670} & \topone{0.9563} & \topone{0.9616}\\

    \midrule
              
       100*100  & 0.9654 & 0.9523 & 0.9588\\

    \bottomrule
		
	\end{tabular}
	}
	}
}
\vspace{-15pt}
\caption{Exploiting the optimal crop size when the deviation distance is 10 pixels. In this work, we try the crop size: 40*40, 60*60, 80*80, 100*100, and no crop.}
\label{tab:crop_size}
\end{table*}

%---------------------------

%---------------------------------------------------------

%--------------------------------------------------------- Exploit the intensity
\section{Exploit the intensity}
\label{subsec:intensity}

\subsection{Fill the cropped area with fixed intensity}
\label{subsec:intensity_fixe}

In addition to the crop size, the crop intensity also has a big influence on the prediction result of HSDN. In this work, we conduct a series of experiments to exploit the optimal crop intensity. Specifically, we use the fixed intensities 0, 128, and 255. Based on the discussion in \secref{subsec:crop}, using crop size 80*80 can reach the best F-score. Therefore, we only consider the crop size 80*80 here. The visualization results of different crop intensity are shown in \figref{fig:crop_intensity}. We also evaluate the Recall, Precision, and F-score with the different intensities. From \figref{fig:intensity_curve} we find that with the intensity 0, it can get the best F-score. Finally, we choose the intensity 0 in this work.

\begin{figure}[h!]
  \includegraphics[width=1\textwidth]{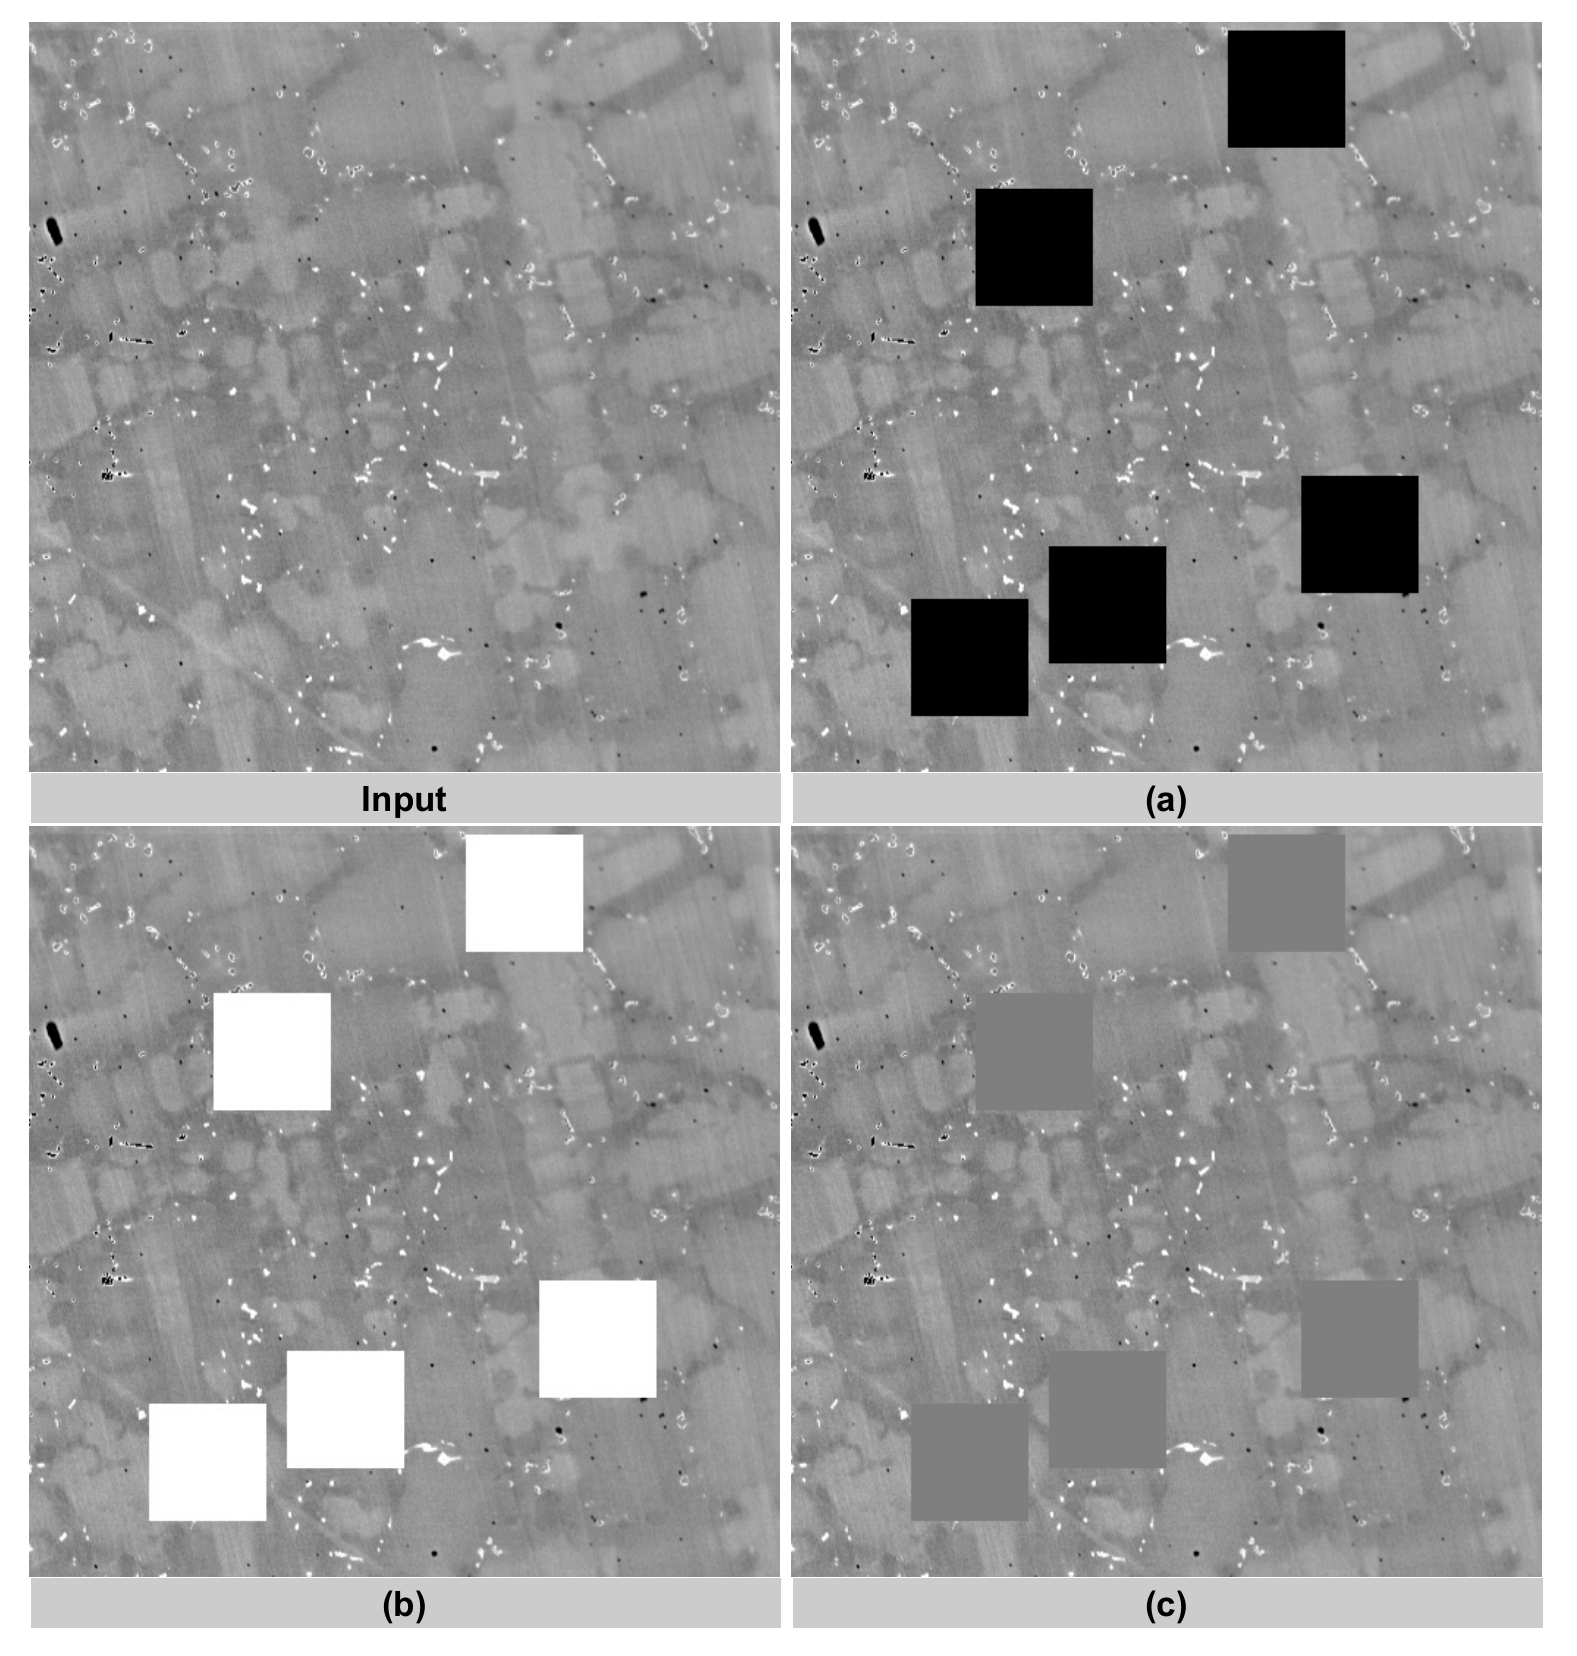}
  \vspace{-25pt}
  \caption{Exploiting the optimal intensity to fill the cropped area. The intensity in the cropped areas is 0 for (a), 255 for (b), and 128 for (c).}
  \label{fig:crop_intensity}
\end{figure}

\begin{figure}[h!]
  \includegraphics[width=1\textwidth]{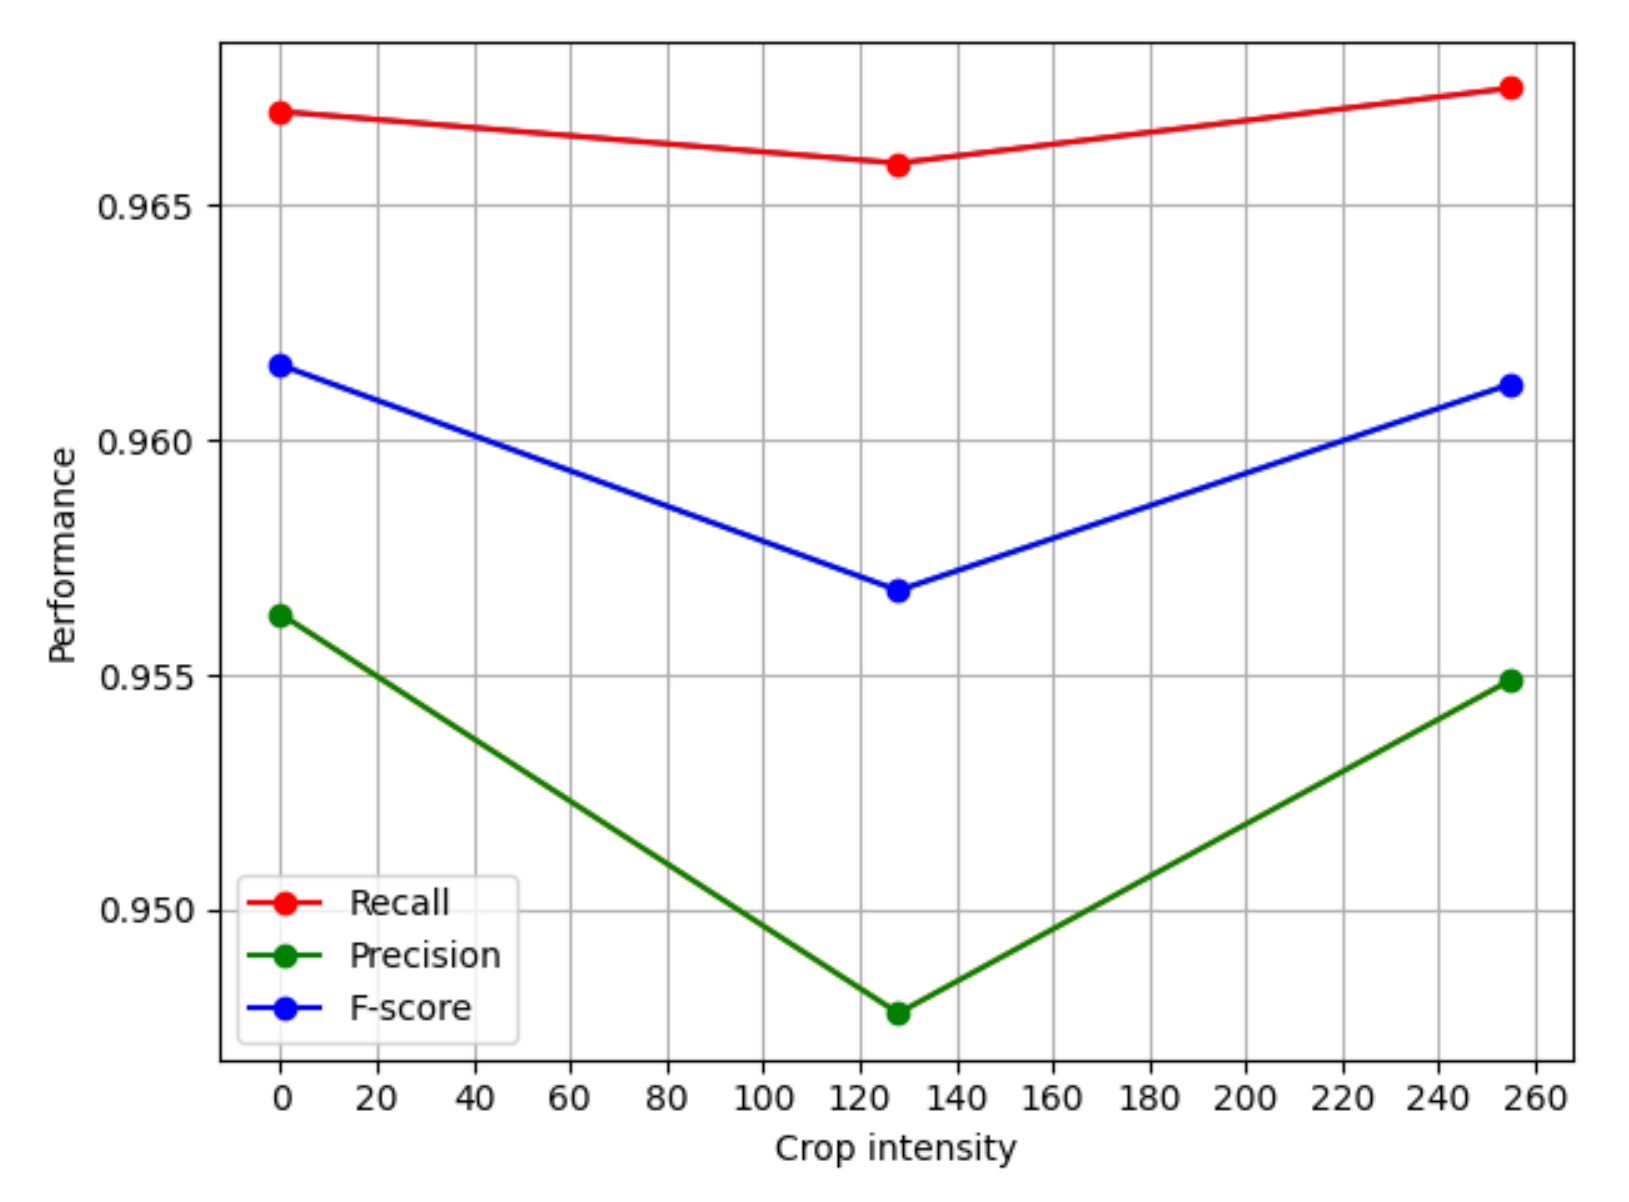}
  \vspace{-25pt}
\caption{Exploiting the optimal intensity to fill the cropped area. In this work, we trial three intensities 0, 128, and 255. Red points denote the Recall, green points denote the Precision, and blue points denote the F-score. When the intensity is equal to 0, it gets the best F-score.}
  \label{fig:intensity_curve}
\end{figure}

\subsection{Process the cropped area with Gaussian blur}

In addition to filling the cropped area with the fixed intensity, we also exploit using the Gaussian blur to process the cropped area. Based on the discussion in \secref{subsec:intensity_fixe}, using the intensity 0, the HSDN can get the best F-score. Therefore, we use the Gaussian blur to process the edges of the cropped areas with intensity 0. The visualization results are shown in \figref{fig:gaussian_sample} (a). Besides, we have a trial to process the cropped areas only with Gaussian blur. The visualization results are shown in \figref{fig:gaussian_sample} (b). From \tableref{tab:intensity} we can see that with the fixed intensity 0, it can get the best F-score.

\begin{figure}[h!]
  \includegraphics[width=1\textwidth]{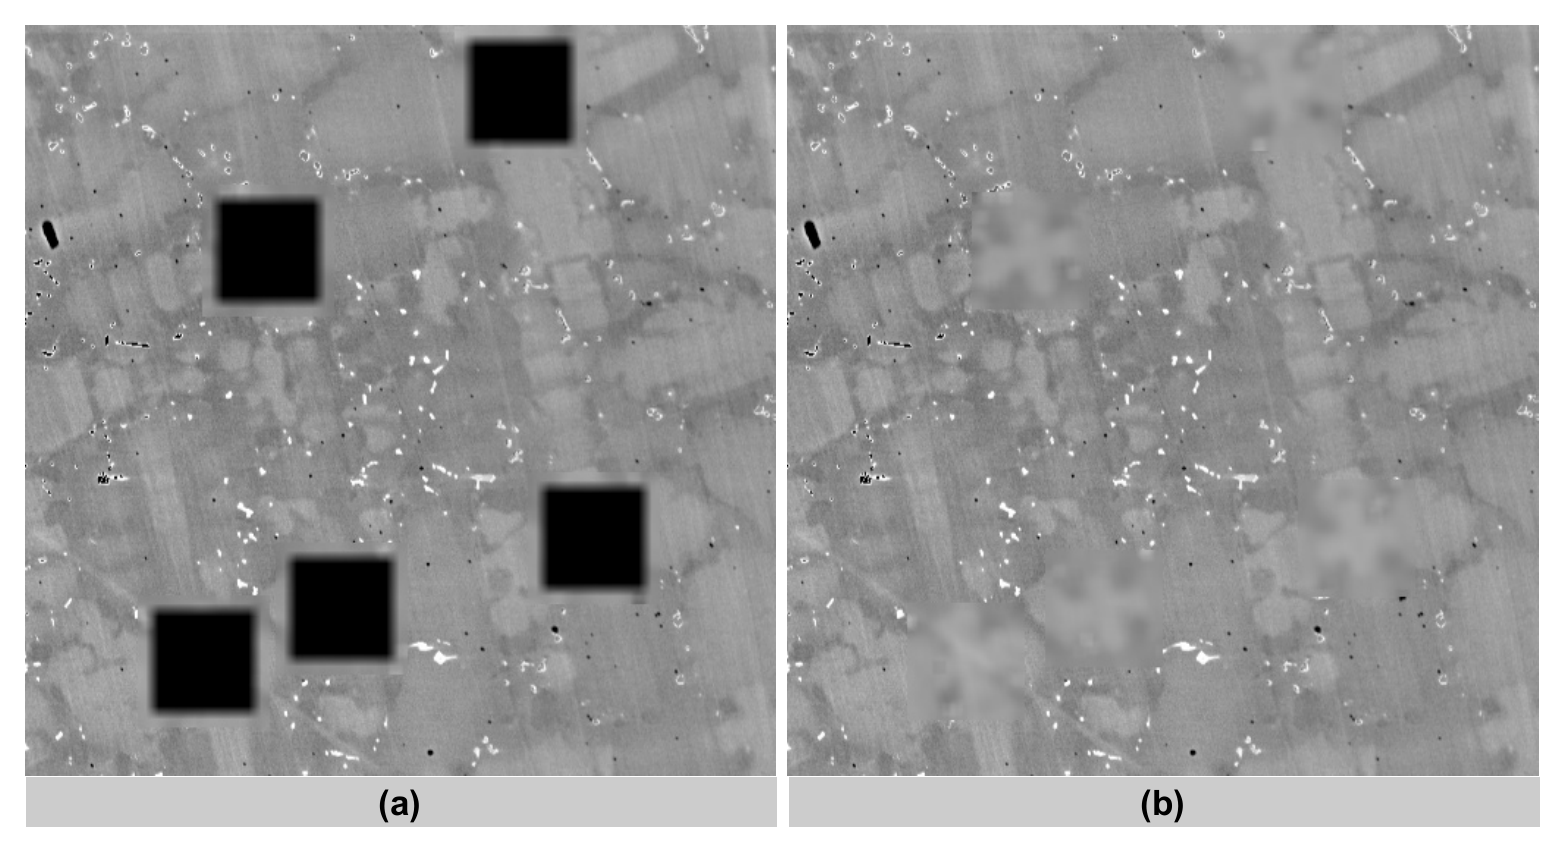}
  \vspace{-25pt}
\caption{Using Gaussian blur to process cropped areas. (a) denotes first to fill the cropped area with intensity 0 and then use Gaussian blur to process the edges. (b) denotes process the cropped areas by Gaussian blur directly.}
  \label{fig:gaussian_sample}
\end{figure}

%-----------intensity----------------
\begin{table*}
\centering
\small
{
    \resizebox{0.8\linewidth}{!}{
    {
	\begin{tabular}{l|c|c|c}
		
    \toprule
      \multicolumn{1}{l|}{intensity} & \multicolumn{1}{c|}{Recall$\uparrow$} & \multicolumn{1}{c|}{Precision$\uparrow$}  & \multicolumn{1}{c}{F-Score$\uparrow$}  \\
    
    \midrule
 
      \topone{0}  & \topone{0.9670} & \topone{0.9563} & \topone{0.9616}\\
   
   \midrule
             
       128  & 0.9659 & 0.9478 & 0.9568\\

    \midrule
             
       255  & 0.9675 & 0.9549 & 0.9612\\

   \midrule
             
       Gaussian & 0.9617 & 0.9597 & 0.9607\\ 

    \midrule
            
       0 + Gaussian  & 0.9617 & 0.9541 & 0.9579\\

    \bottomrule
		
	\end{tabular}
	}
	}
}
\vspace{-15pt}
\caption{Exploiting the optimal intensity in the cropped areas when deviation distance is 10 pixels and cropped size is 80*80. 0 + Gaussian means first filling the cropped areas with intensity 0 and then processing the edges by Gaussian blur.}
\label{tab:intensity}
\end{table*}
%---------------------------
